# Supplementary material for: COVID-19: Tail Risk and Predictive Regressions
Source: arXiv:2009.02486 source file (2021-10-13)
Supplement: Supplementary file 1 [file appendix.tex]

\section{t-statistics}

\begin{table}[h] \centering 
	\caption{Ripple and stock factors} 
	\label{} 
	\scalebox{0.6}{
		\begin{tabular}{@{\extracolsep{5pt}}lccccc} 
			\\[-1.8ex]\hline 
			\hline \\[-1.8ex] 
			& \multicolumn{5}{c}{\textit{$(R_{t}-$risk-free return}$)$} \\ 
			\\[-1.8ex] & CAPM & 3-F & 4-F & 5-F & 6-F\\ 
			\hline \\[-1.8ex]
			Mkt.RF & $-$0.142 & $-$0.138 & $-$0.134 & $-$0.147 & $-$0.137 \\ 
			& [1.213] & [1.104] & [1.139] & [0.927] & [0.974] \\ 
			& ($-$0.267) & ($-$0.247) & ($-$0.234) & ($-$0.236) & ($-$0.224) \\ 
			  &\{0.154\}&\{$-$0.146\}&\{$-$0.417\}&\{0.111\}&\{$-$0.442\}\\
			SMB  &  & 0.191 & 0.210 & $-$0.090 & $-$0.057 \\ 
			&  & [0.822] & [0.912] & [0.318] & [0.434] \\ 
			&  & (0.221) & (0.234) & ($-$0.099) & ($-$0.061) \\ 
			  
			  &&\{$-$0.009\}&\{$-$0.109\}&\{$-$0.371\}&\{$-$0.461\}\\
			HML &  & $-$1.076 & $-$1.040 & $-$1.728$^{*}$ & $-$1.672$^{*}$ \\ 
			&  & [0.068] & [0.254] & [$-$0.733] & [$-$0.544] \\ 
			&  & ($-$1.406) & ($-$1.295) & ($-$1.945) & ($-$1.849) \\ 
			  
			  &&\{$-$2.812\}&\{$-$2.027\}&\{$-$2.209\}&\{$-$1.965\}\\
			MOM &  &  & 0.001 &  & 0.001 \\ 
			&  &  & [0.509] &  & [0.609] \\ 
			&  &  & (0.141) &  & (0.255) \\ 
			 
			  &&&\{$-$0.587\}&&\{0.158\}\\
			RMW &  &  &  & $-$1.406 & $-$1.410 \\
			&  &  &  &[$-$1.640] & [$-$1.649] \\ 
			&  &  &  & ($-$1.137) & ($-$1.135) \\ 
		
			  &&&&\{$-$1.246\}&\{$-$1.232\}\\
			CMA&  &  &  & 1.562 & 1.589 \\ 
			&  &  &  & [1.180] & [1.217] \\
			&  &  &  & (1.212) & (1.261) \\ 
			 
			  &&&&\{1.610\}&\{1.701\}\\
			Alpha  & 0.015 & 0.015 & 0.015 & 0.015 & 0.015 \\
			&[2.926$^{*}$] & [2.920$^{*}$] & [2.901$^{*}$] & [3.012$^{*}$] & [2.991$^{*}$] \\ 
			& (3.175$^{*}$) & (3.769$^{*}$) & (3.395$^{*}$) & (3.525$^{*}$) & (3.306$^{*}$) \\ 
			  
    			  &\{4.303$^{*}$\}&\{4.508$^{*}$\}&\{4.426$^{*}$\}&\{4.366$^{*}$\}&\{4.239$^{*}$\}\\
			\\[-1.8ex]
			\hline 
			\hline   
	\end{tabular} }
\end{table}

\begin{table}[h!] \centering 
	\caption{Ethereum and stock factors} 
	\label{} 
	\scalebox{0.6}{
		\begin{tabular}{@{\extracolsep{5pt}}lccccc} 
			\\[-1.8ex]\hline 
			\hline \\[-1.8ex] 
			& \multicolumn{5}{c}{\textit{$(R_{t}-$risk-free return}$)$} \\ 
			\\[-1.8ex] & CAPM & 3-F & 4-F & 5-F & 6-F\\ 
			\hline \\[-1.8ex] 
			Mkt.RF & $-$0.542 & $-$0.527 & $-$0.506 & $-$0.529 & $-$0.495 \\ 
			& ($-$0.780) & ($-$0.800) & ($-$0.782) & ($-$0.776) & ($-$0.738) \\ 
			  & [0.029] & [0.288] &[0.516] & [0.298] & [0.590] \\ 
			  &\{0.005\}&\{$-$0.444\}&\{$-$0.484\}&\{$-$0.670\}&\{$-$0.733\}\\
			SMB &  & $-$0.022 & 0.093 & $-$0.257 & $-$0.128 \\
			&  & ($-$0.029) & (0.120) & ($-$0.324) & ($-$0.160) \\ 
			  &  & [$-$1.644] & [$-$1.005] &[$-$1.896] & [$-$1.267] \\ 
			  			  &&\{0.163\}&\{$-$0.075\}&\{0.116\}&\{$-$0.064\}\\
			HML &  & $-$0.460 & $-$0.300 & $-$1.103 & $-$0.958 \\ 
			&  & ($-$0.543) & ($-$0.379) & ($-$1.094) & ($-$1.048) \\ 
			  &  & [$-$0.869] & [0.009] & [$-$1.351] & [$-$0.767] \\ 
			  			  &&\{$-$0.320\}&\{$-$0.573\}&\{$-$0.438\}&\{$-$0.534\}\\
			MOM &  &  & 0.003 &  & 0.004 \\
			&  &  & (0.634) &  & (0.720) \\ 
			  &  &  & [2.518] &  & [2.640] \\ 
			  			  &&&\{$-$3.534\}&&\{$-$1.037\}\\
			RMW &  &  &  & $-$1.227 & $-$1.224 \\
			&  &  &  & ($-$1.151) & ($-$1.145) \\ 
			  &  &  &  & [$-$0.927] & [$-$0.932] \\ 
			  			  &&&&\{$-$0.202\}&\{$-$0.171\}\\
			CMA &  &  &  & 1.567 & 1.677 \\ 
			&  &  &  & (1.142) & (1.181) \\ 
			  &  &  &  & [1.029] &[1.301] \\ 
			  			  &&&&\{$-$0.083\}&\{$-$0.061\}\\
			Alpha& 0.013& 0.013 & 0.013 & 0.014 & 0.014\\ 
			& (3.426$^{*}$) & (3.586$^{*}$) & (3.499$^{*}$) & (3.731$^{*}$) & (3.555$^{*}$) \\ 
			 & [3.393$^{*}$] & [3.418$^{*}$] & [3.389$^{*}$] &[3.474$^{*}$] & [3.450$^{*}$] \\ 
			 			  &\{2.478\}&\{2.259\}&\{2.327\}&\{2.364\}&\{2.374\}\\
			\\[-1.8ex]
			\hline 
			\hline   
	\end{tabular} }
\end{table}
